# Supplementary material for: Temporal Linear Item-Item Model for Sequential Recommendation
Source: arXiv:2412.07382 source file (2024-12-10)
Supplement: Supplementary file 1 [file tab-appendix-ablation_perform.tex]

\begin{table} \small
\caption{Ablation study of TALE on ML-1M and Beauty. TALE consists of three parts: (1) time interval-aware weighting, (2) trend-aware normalization, and (3) single-target augmentation. Each metric is NDCG@5.}
\label{tab:ablation_performance_appen}
\vspace{-2mm}
\begin{center}
 % 테이블 행 간격
\begin{tabular}{P{0.25cm}P{0.25cm}P{0.25cm}|P{0.75cm}P{0.75cm}P{0.75cm}|P{0.75cm}P{0.75cm}P{0.75cm}}
\toprule
\multicolumn{3}{c|}{Dataset}         & \multicolumn{3}{c|}{ML-1M}          & \multicolumn{3}{c}{Beauty}              \\
(1) & (2) & (3)   & N@5   & Tail & Head  & N@5   & Tail & Head \\
\midrule

\cmark & \cmark & \cmark   & \textbf{0.1276} & \textbf{0.0814} & \textbf{0.1614}   & \textbf{0.0482}   & \textbf{0.0271} & \underline{0.0736}     \\
- & \cmark & \cmark   & 0.1227  & 0.0739 & 0.0661 & 0.0450  & 0.0239 & 0.0487     \\
\cmark & - & \cmark   & \underline{0.1257}  & \underline{0.0773} & 0.1573 & \underline{0.0468}  & \underline{0.0243} & 0.0659       \\
\cmark & \cmark & -   & 0.0473  & 0.0161 & 0.1528 & 0.0296  & 0.0154 & 0.0696    \\
- & - & \cmark   & 0.1172  & 0.0685 & 0.0701 & 0.0444 & 0.0235  & 0.0467    \\
- & \cmark & -   & 0.1187  & 0.0659 & \underline{0.1611} & 0.0431  & 0.0242  & \textbf{0.0739} \\
\cmark & - & -   & 0.0430  & 0.0114 & 0.1584 & 0.0303  & 0.0150  & 0.0704 \\
- & - & -   & 0.1164  & 0.0624 & 0.1559 & 0.0435  & 0.0235  & 0.0676 \\

\bottomrule
\end{tabular}
% \vspace{-4mm}
\end{center}
\end{table}
