# Supplementary material for: Temporal Linear Item-Item Model for Sequential Recommendation
Source: arXiv:2412.07382 source file (2024-12-10)
Supplement: Supplementary file 2 [file tab-appendix-c.tex]

\begin{figure}
\begin{tabular}{ccc}
\includegraphics[height=2cm]{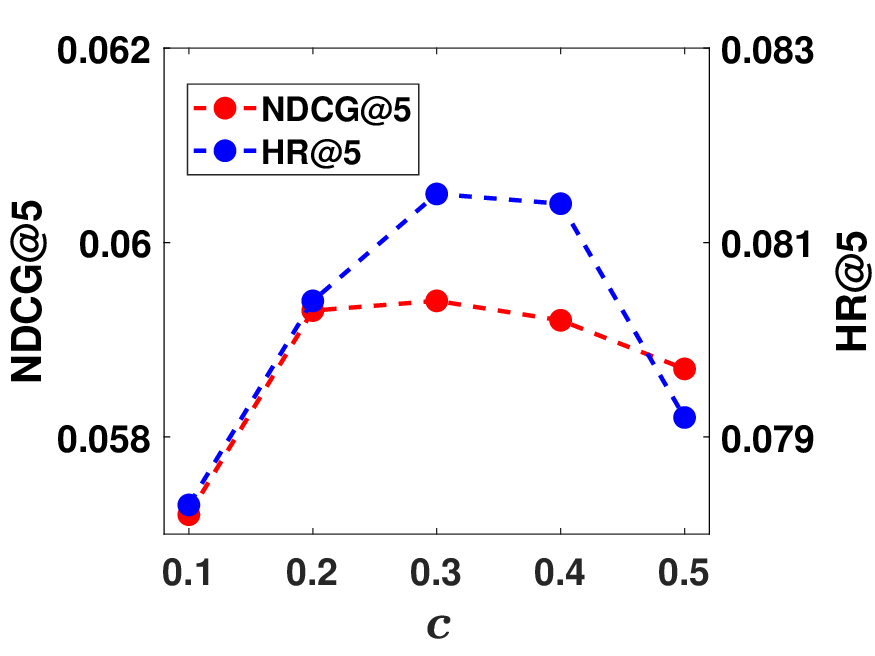} &
\includegraphics[height=2cm]{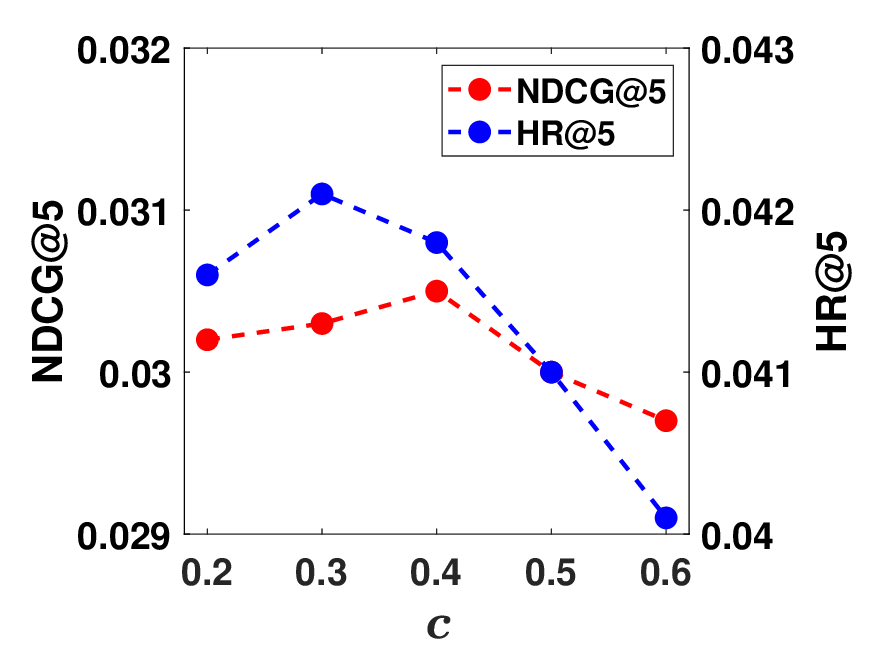} &
\includegraphics[height=2cm]{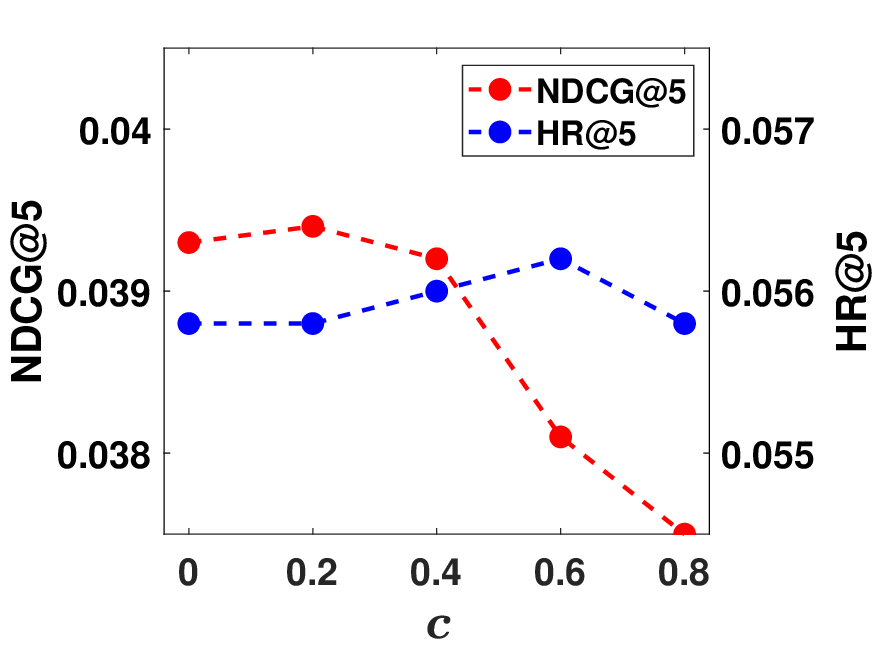}\\
\multicolumn{1}{c}{(a) Toys} & \multicolumn{1}{c}{(b) Sports} & \multicolumn{1}{c}{(c) Yelp} \\
\end{tabular}
\vspace{-2mm}
\caption{Performance of TALE over $c$ for time interval-aware weighting on Toys, Sports, and Yelp. }\label{fig:c_appen}

% \vspace{-3mm}
\end{figure}
